# Supplementary material for: UTFix: Change Aware Unit Test Repairing using LLM
Source: arXiv:2503.14924 source file (2025-03-19)
Supplement: Supplementary file 1 [file appendix.tex]

\section{Appendix}

% \begin{figure}[h]
%     \centering
%     \includegraphics[width=\linewidth]{figure/Error-Message.png}
%     \caption{Assertion Failure}
%     \label{fig:errormessage}
% \end{figure}
